# Supplementary material for: Polymerization and replication of primordial RNA induced by clay-water interface dynamics
Source: arXiv:2411.05795 source file (2025-09-15)
Supplement: Supplementary file 1 [file alejandre_et_al_SI.pdf]

---

# SUPPORTING INFORMATION FOR “POLYMERIZATION AND REPLICATION OF PRIMORDIAL RNA INDUCED BY CLAY-WATER INTERFACE DYNAMICS”

---

Carla Alejandre, Adrián Aguirre-Tamaral, Carlos Briones and Jacobo Aguirre

## S1. EarlyWorld’s algorithm

### A. Definitions and basic rules of the model

EarlyWorld is a computational environment that simulates, in a simplified, stochastic and discrete-time manner, the non-enzymatic polymerization and template-dependent replication of RNA on a clay-water interface. More precisely, ribonucleotides (nts), single stranded (ss) and double stranded (ds) RNA molecules move from an aqueous solution (the pool from now on) to the surface of a clay, and vice versa.

There is a total absence of catalytic molecules such as ribozymes or protein enzymes (e.g., RNA polymerases). Also, ssRNA molecules are not allowed to auto-hybridize forming secondary structures. Additionally, any genetic alphabet can be defined in EarlyWorld by the number of different nts and its base-pairing rules.

Dynamics in EarlyWorld takes place in two separated compartments, comp.I and comp.II, each of them representing a different microenvironment of the clay-water interface [1, 2, 3, 4], and whose simulations run independently. Three levels are relevant for the evolution of the system: the clay or level 0, where nts and polymers can be adsorbed—described by a 1D-vector of length  $L$ — (both in comp.I and comp.II); the complementary level or level 1, where nts can only be placed if they are complementary to those of the template ssRNA placed in level 0 and contribute to the formation of dsRNA molecules via hydrogen bonding—described by a 1D-vector of length  $L$ — (only in comp.II); and the aqueous phase, pool or level 2, represented by a *disordered box* where an unlimited number of free nts, ssRNA and dsRNA molecules stay in solution (both in comp.I and comp.II, dsRNA molecules only in the latter). See Fig. S10 for different clay scenarios to the ones described here.

The system’s performance depends on two main parameters:  $\alpha$  describes the strength of the clay-nt interactions—known to be ionic bonds and weak Van der Waal forces [5, 6, 3]—, and  $\beta$  describes the strength of nt-nt interactions—due to hydrogen bonding between nucleobases— [7]. Both quantities depend on the environment that surrounds them.

Simulations in compartments I and II start with a fixed number  $N$  of initial nts floating freely in the pool. Unless said otherwise, a clay of length  $L = 200$  positions was used (a length sufficiently large to accommodate several small RNA oligomers, while keeping simulations computationally affordable) and an alphabet of four different nts (A4) displaying the canonical base-pairing rules ( $A=U$  and  $G=C$ ), with  $N = 1600$  nts equally distributed between A, U, G and C, so that their abundances were not a limiting factor. Simulations stop when the simulation time  $t_{\max}$  is reached. Throughout the calculations in this work,  $t_{\max} = 2 \times 10^4$  except when the dependence of the system on the simulation time is particularly studied (see Fig. S3).

The steps of the algorithm at each time step are similar in both compartments and are summarized as follows:

- A molecule (nt, ssRNA or dsRNA, the latter only in comp.II) selected from the pool falls into the clay.
- Attending to the rules described below in sections S1.B and S1.C, the molecule either (i) remains adsorbed to the clay (level 0), (ii) is hybridized to other nt or ssRNA if they are complementary (level 1, only in comp.II), or (iii) returns to the pool (level 2) with no changes. In the case it remains attached to level 0 or 1, either random or template-dependent polymerization can occur, respectively.

- The breakage probability of all the existing non-covalent interactions in the system (desorption probability in clay-nt interactions and denaturation probability in nt-nt interactions) in that time step is evaluated. As a consequence, some molecules may be released from levels 0 or 1 and return to level 2 (the pool).
- The simulation is repeated  $t_{\max}$  time steps, and then stops.

## B. Detailed description of compartment I simulations

Comp.I represents a clay internal channel or interlayer that is wide enough to accommodate ssRNA molecules, but not dsRNA molecules. Here, random polymerization of nts takes place due to the catalytic action of the clay, but complementary base pairing between nts is not possible.

Simulations start with  $N$  initial nts floating in the pool, as described in section S1.A, and the clay level completely empty. At each time step of the simulation, the system follows the steps depicted in the flow diagram on Fig. S1. As time passes, ssRNA polymers are formed on the clay, desorb and move to the pool (thus enriching it in larger oligomers), and can also be adsorbed again on the clay surface and continue polymerizing. Simulations stop when the simulation time  $t_{\max}$  is reached. Besides the detailed flow chart of Fig. S1, important considerations are clarified below:

- The molecule  $\mathcal{M}$  (that can be a nt or a ssRNA oligomer) selected at time step  $k$  to interact with the clay is chosen randomly from all the molecules in the pool with the weighted probability

$$P_k(\mathcal{M}) = \text{length}(\mathcal{M})/S_k, \quad (1)$$

where  $S_k$  is the sum of all molecule lengths (computed as their number of nts) present in the pool in time step  $k$ . Therefore, larger polymers have more chances to be adsorbed to the clay, as we assume they diffuse slower and establish more interactions with the substrate than smaller oligomers.

- A randomly chosen nt of the selected molecule interacts with a randomly chosen empty position of the clay. The number of positions in the clay that interact with the falling molecule is equal to its length.
- The place on the clay where  $\mathcal{M}$  falls is considered empty only if all the individual positions with which the molecule interacts are empty and the whole molecule falls inside the boundaries of the  $L$  clay positions.

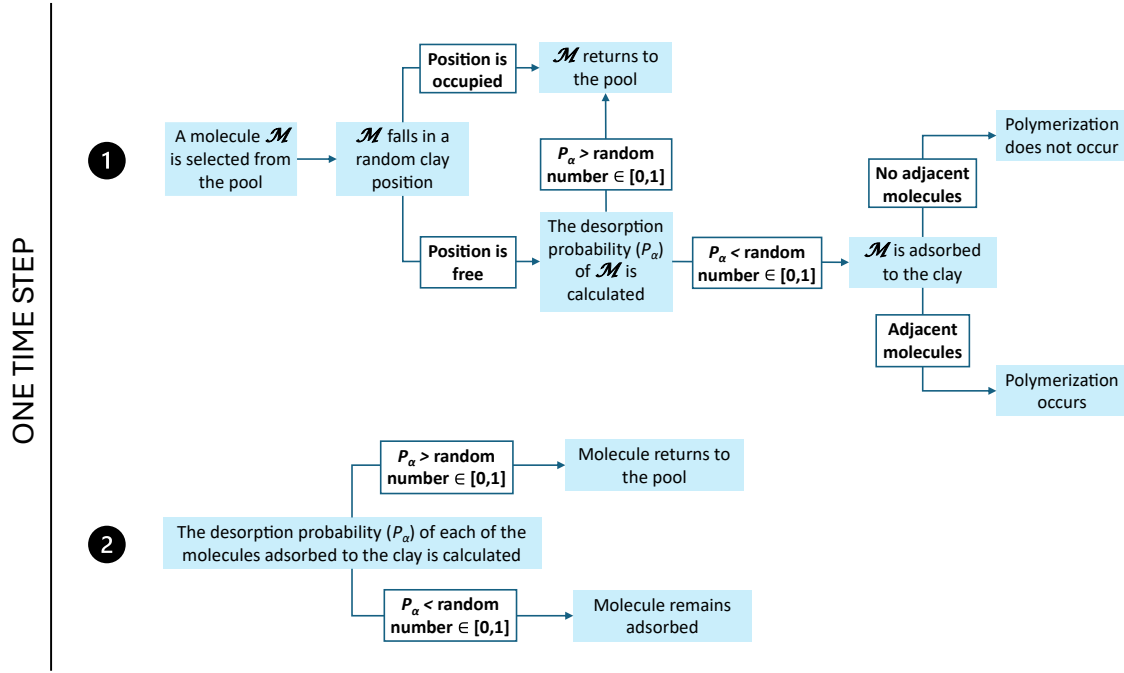

Figure S1: Flow diagram of compartment I simulations. The chart describes the steps followed by the computational algorithm for every time step of a simulation. Two major processes take place in each time step: 1) The dynamics of the molecule  $\mathcal{M}$  that falls into the clay, and 2) the dynamics of the rest of nts and ssRNA molecules that are attached to the clay.

- $P_\alpha$  is the desorption probability and is calculated as

$$P_\alpha = e^{-l\alpha}, \quad (2)$$

where  $l$  stands for the polymer's length and  $\alpha > 0$  describes the strength of the clay-nt interactions in the environment that surrounds them. Note that the ssRNA oligomers are attached or detached from the clay along their entire length: this model does not consider partially adsorbed/desorbed molecules. In consequence, Eq. 2 can be interpreted as a Bernoulli random process, where the polymer desorbs from the clay only if all outcomes are successful.

- If polymerization occurs,  $\mathcal{M}$  forms a covalent bond with one nt at any of its two adjacent positions, producing a longer polymer that is yet attached to the clay until its desorption probability is again evaluated. Throughout the entire simulation, the covalent sugar-phosphate backbone of the polymers remains unbreakable (i.e., RNA hydrolysis is not considered in this model, except when we explicitly study the influence of hydrolysis in the system, see section Results "Compartment II: Template-dependent RNA replication on a clay surface" of the main text and Fig. S8).

### C. Detailed description of compartment II simulations

Comp.II represents wide clay channels that can accommodate both ssRNA and dsRNA molecules, as well as inter-particle sites and external clay surfaces. Therefore, here both random polymerization of nts (as in comp.I) and template-dependent RNA replication can occur.

Simulations start with an initial ssRNA of 20 nts in length that represents a polymer formerly produced in comp.I, which has been pushed out of it to eventually enter comp.II, and has finally been adsorbed to its clay. The composition and sequence of this original polymer (strand O from now on) is set randomly at the beginning of each simulation, as well as the clay position of comp.II where it is initially adsorbed. The rest of the initial conditions are the same as in comp.I: simulations start with  $N$  initial nts floating in the pool and the clay level completely empty except for the initial O polymer.

At each time step of the simulation, the system follows the flow diagram shown in Fig. S2. As time passes, polymers form and the pool becomes enriched in larger molecules (both ssRNA and dsRNA molecules), that can also be adsorbed again to the clay or, only in the case of ssRNA, be hybridized to other ssRNA at the complementary level or level 1. RNA molecules can form by random polymerization on the clay surface (as it happens in comp.I), but also by template-dependent polymerization (exclusive of comp.II). Thus, during each simulation, the dynamics produces complementary C and replicate R (i.e., complementary to C) strands of the original O, as well as other newly-generated random sequences  $O_{\text{new}}$  than can also be copied in their complementary  $C_{\text{new}}$  and replicate  $R_{\text{new}}$  strands. Only C and R strands of the original O are plotted in the figures of this work, as  $C_{\text{new}}$  and  $R_{\text{new}}$  do not proceed from the original ssRNA oligomer O. Finally, simulations stop after  $t_{\text{max}}$  time steps.

Besides the detailed flow chart of Fig. S2, important considerations are clarified below:

- The molecule  $\mathcal{M}$  (which can be a nt, a ssRNA or a dsRNA) selected in the pool and the position of the clay (levels 0 or 1) where it adsorbs are chosen in the same way as in comp.I, section S1.B. When dsRNA molecules are formed, their length (used to compute  $P_k(\mathcal{M})$  in Eq. 1) is calculated as the sum of the lengths of the two strands that compose the duplex.
- In comp.II, nts and ssRNA molecules can be adsorbed to the clay (level 0) or be hybridized to a template strand (level 1), the latter happening only if they are fully complementary (mutations or nucleotide mismatches are not accepted in this model). On the contrary, dsRNA molecules can exclusively be adsorbed to the clay (level 0).
- As in comp.I, the place where  $\mathcal{M}$  adsorbs is considered empty only if all the positions where the molecule falls (in level 0 or in level 1, depending on the case) are empty and the whole oligomer fits inside the boundaries of the  $L$  positions.
- The desorption probability is calculated as in comp.I, Eq. 2.
- The denaturation probability  $P_\beta$  is

$$P_\beta = e^{-l\beta}, \quad (3)$$

where  $l$  stands for the dsRNA length and  $\beta > 0$  describes the strength of nt-nt interactions in the environment that surrounds them. As it happened with ssRNA molecules adsorbed/desorbed from the clay, ssRNA molecules hybridize and denature from the templates along their entire length: molecules partially hybridized/denatured are not allowed. In consequence, Eq. 3 can also be interpreted as a Bernoulli random process, where the ssRNA denatures from the template only if all outcomes are successful.

- Polymerization occurs as explained for comp.I, section S1.B, but in this case it can take place at both levels: 0 or 1, the latter being a template-dependent polymerization.

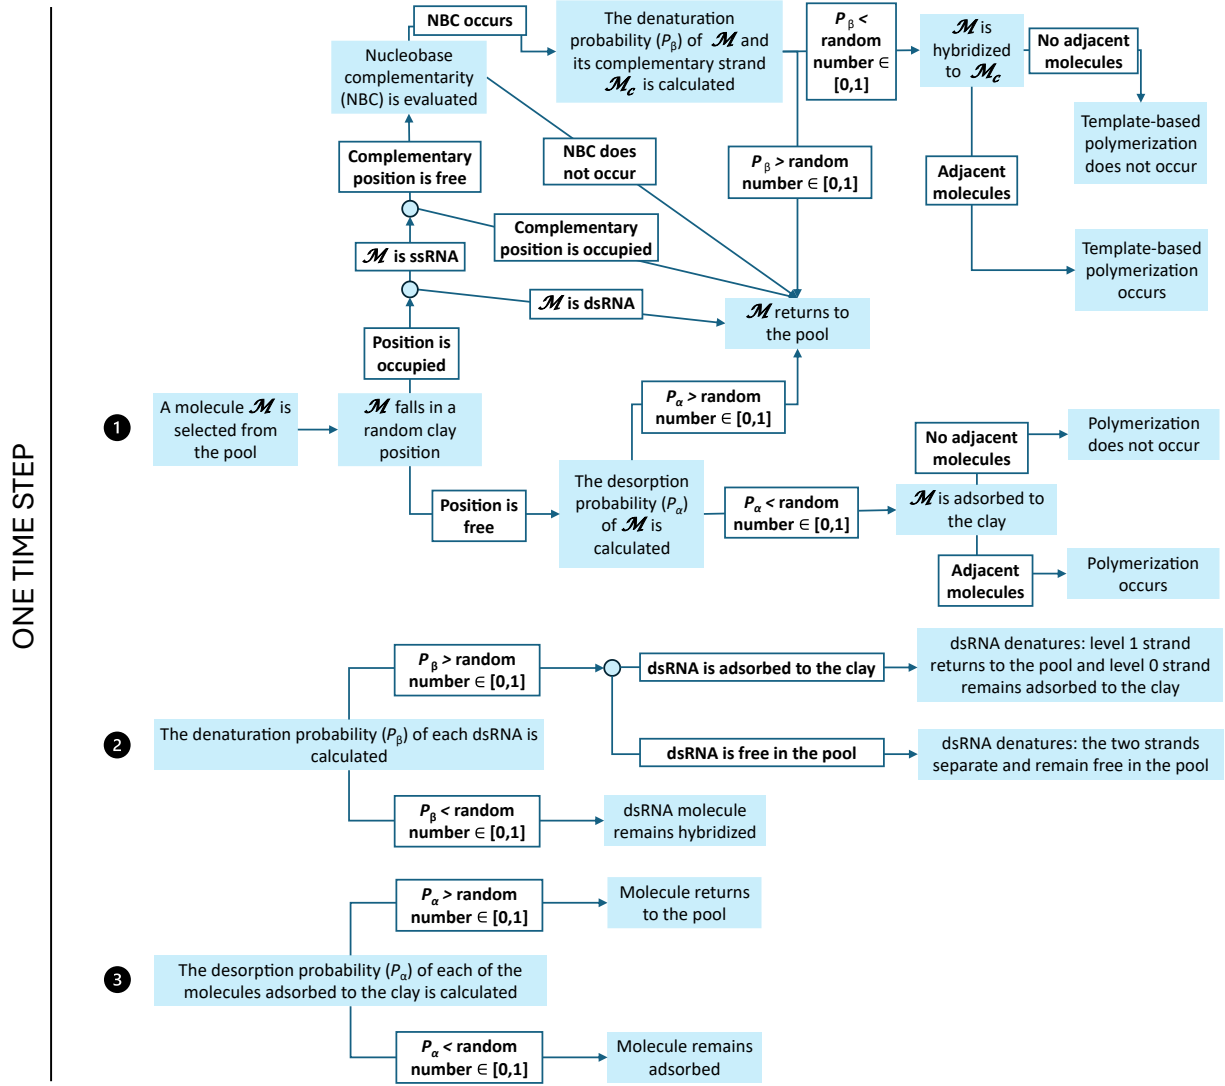

Figure S2: Flow diagram of compartment II simulations. The chart describes the steps followed by the computational algorithm for every time step of a simulation. Three major processes take place in each time step: 1) The dynamics of the molecule  $\mathcal{M}$  that is adsorbed to the clay, 2) the dynamics of all the dsRNA molecules both attached to the clay and floating in the pool (in the latter case, whether they remain hybridized or denature), and 3) the dynamics of all the nts, ssRNA and dsRNA molecules that are attached to the clay (whether they remain adsorbed or they desorb and return to the pool).

## S2. Calculation of maximum polymer lengths

Most of the computational results displayed in the main text represent statistical measures of the distribution of maximum polymer lengths obtained along every realization for a concrete number of realizations (typically 100), each of them running for a limited number of time steps  $t_{\max}$ . Simulations are stochastic, therefore each of them represents a different trajectory and, in the case of comp.II, the original ssRNA sequence of 20 nts in length is randomly created at the beginning of every realization.

In comp.I, the maximum polymer length measured in one realization of the process represents the longest polymer formed by adsorption of nts on the clay, which is later on released to the pool at any time step. Notice that even longer polymers attached to the clay may form, but will not be considered until they are detached from the surface.

In comp.II, the maximum polymer lengths measured in one realization of the process are calculated as the lengths of the longest complementary C and replicate R polymers denatured from their templates and released to the pool at any time step.

## S3. Sequence accuracy

Complementary C and replicate R molecules of the original O sequence can be “contaminated” at their ends with other added nts or ligated ssRNA molecules, as RNA ligation (either produced —randomly— at level 0 or—in a template-dependent manner— at level 1) is based on the same process of phosphodiester bond formation that is involved in RNA polymerization. As a result, C or R molecules are frequently found to be elongated with random sequences covalently linked to their ends, which are not related to the original molecule O and give rise to chimeric sequences [8]. In order to measure this phenomenon, we define the accuracy of a sequence  $s$  of type C or R of length  $l_s$  as

$$A_s = 100 \times \frac{l_O}{l_s}, \quad (4)$$

where  $l_O$  is the number of nts of sequence  $s$  that are (i) complementary to a fraction (or the totality) of the original sequence O in a ssRNA of type C, or (ii) equal to a fraction (or the totality) of the original sequence O in a ssRNA of type R.

To avoid the loss of identity of the original O sequences, the C and R molecules resulting from simulations are only counted if they have an accuracy of  $>75\%$ , i.e., their sequences must be formed by  $>75\%$  of products of the copied polymer O. In practice, this means that each replicated ssRNA molecule can be up to 33% longer than the product of the original O it contains. As in the model RNA polymers cannot be degraded or split into shorter oligomers (except when we explicitly study the influence of hydrolysis in the system, see section Results “Compartment II: Template-dependent RNA replication on a clay surface” of the main text), such additional nts that are allowed to decrease the accuracy of the copied molecule up to 75% appear at its ends but not at internal positions of the sequence.

For the sake of clarity, we provide here an example of the meaning of the accuracy of a sequence in EarlyWorld: when a simulation in comp.II produces a maximum length of an R molecule equal to 20 nts, with accuracy of  $>75\%$ , it means that the replicated sequence has a core of 20 nts that is an exact copy of the original O, but it can show up to 6 spurious nts covalently bound to its ends (i.e.,  $20 \leq l_s \leq 26$  nts). In turn, an accuracy of 100% means that R is 20 nts long and its sequence is identical to that of O.

Figure S3 shows the maximum C (green) and R (purple) polymer length distributions for different simulation times  $t_{\max}$ , with an accuracy of  $>75\%$  (i.e., the accuracy allowed in this work) in Fig. S3A, and of 100% in Fig. S3B. Importantly, EarlyWorld yields fully accurate (i.e., 100%) C and R sequences of length 20—and therefore R being identical to O—for certain sets of parameters, although their abundance is, obviously, smaller than that of less accurate polymers.

Finally, note that the efficiency of the results obtained saturate beyond a simulation time of  $t_{\max} \sim 2 \cdot 10^4$  time steps for an accuracy of  $>75\%$ . For this reason, we chose such value for the simulations developed in this work.

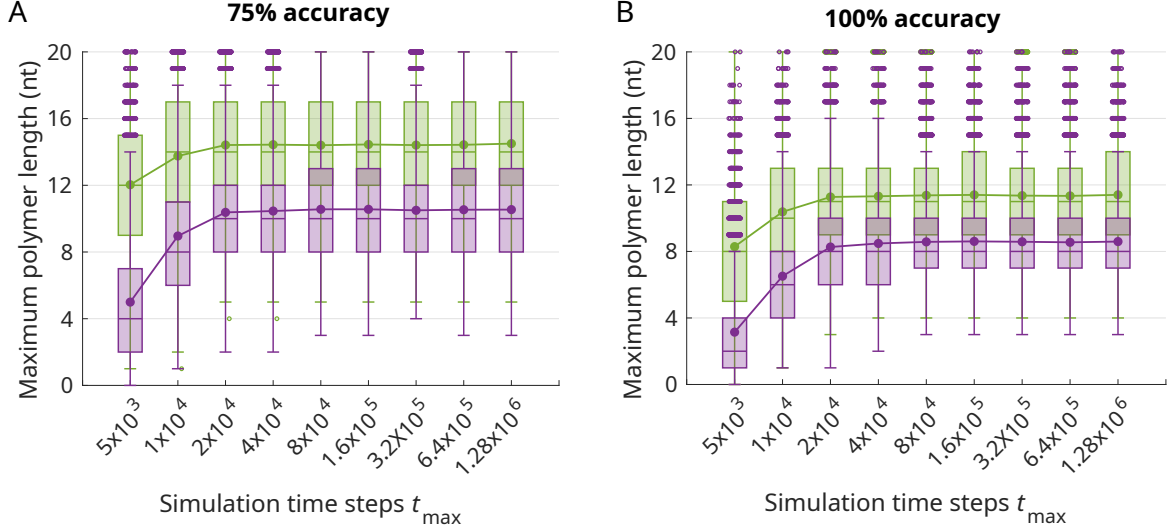

Figure S3: Maximum complementary (C, green) and replicate (R, purple) polymer length distribution for different simulation times. Panel (A) plots replication products with an accuracy of  $>75\%$ , whereas panel (B) shows products with an accuracy of  $100\%$ . Every simulation was repeated  $10^4$  times. Parameters:  $\alpha_0 = 0.6$ ,  $\beta_0 = 7$ ,  $f = 0.99$ ,  $T = T_\alpha = T_\beta = 2500$  (coinciding with the most favorable result in Fig. 4A). Note that throughout the paper simulation times were  $t_{\max} = 2 \times 10^4$  time steps.

#### S4. Analysis of the expansion of sequence space exploration enabled by non-canonical base pairs through the lens of information theory.

The replication space set  $\sigma$  is defined here as the set of complementary sequences (of any length  $> 1$ ) that can be generated from a ssRNA of length  $\mathcal{L}$ . Its cardinal  $|\sigma|$  provides a useful measure of the alphabet's capacity to explore sequence space through template-dependent complementarity. For a canonical (non-degenerated) alphabet of  $\mathcal{A}$  letters, such as A4,  $|\sigma|$  corresponds to the sum of all distinct sequences longer than 1 nt that can be generated from a ssRNA of length  $\mathcal{L}$  nts (i.e., one of length  $\mathcal{L}$ , two of length  $\mathcal{L} - 1$ ...), yielding

$$|\sigma| = \sum_{k=2}^{\mathcal{L}} (\mathcal{L} + 1 - k) = \frac{(\mathcal{L} - 1)\mathcal{L}}{2}. \quad (5)$$

It is well-established that not all base pairs occur with equal frequency in dsRNAs. For instance, wobble UG pairs are weaker than UA ones despite both having two hydrogen bonds, leading to a bias that favors U pairing with A over G. This variability in pairing propensity —i.e., the degree of degeneracy— can be quantified under the lens of information theory. Traditionally, information theory has been applied to measure the average information content per symbol of a ssRNA sequence, using Shannon entropy [9, 10]. However, instead of the information content of a sequence, we want to quantify how the degeneracy of copy can affect the ability to explore the sequence space through replication. For that purpose, we use the binary Shannon entropy of copy per degenerated base  $i$

$$H_i = -p_i \log p_i - (1 - p_i) \log (1 - p_i), \quad (6)$$

that allows to estimate the effective amount of degenerated sequences associated to degenerated base  $i$  as  $\sim 2^{H_i}$  [11]. Therefore, when the alphabet includes a subset of  $d$  degenerated letters (e.g.,  $d = 2$  in A4\*) —each with, in principle, different probabilities  $p_i$  and  $1 - p_i$  of pairing with 2 complementary partners— and assuming these degenerated bases are randomly distributed along the original sequence, a sequence fragment of length  $k$  will contain, on average, a fraction  $k/\mathcal{L}$  of the total degenerated bases per sequence  $\mathcal{L}H/\mathcal{A}$ . This results into a total alphabet degeneracy, obtained from the contributions of the degenerated letters, of  $H = \sum_{i=1}^d H_i$ . Consequently, we can estimate the replication space size as

$$|\sigma| = \sum_{k=2}^{\mathcal{L}} 2^{\frac{kH}{\mathcal{A}}} (\mathcal{L} + 1 - k) = \frac{4^{H/\mathcal{A}}}{(2^{H/\mathcal{A}} - 1)^2} [2^{\mathcal{L}H/\mathcal{A}} - (2^{H/\mathcal{A}} - 1)\mathcal{L} - 1]. \quad (7)$$

Thus, for  $\mathcal{L} \gg 1$ , the size of the non-degenerated replication space  $|\sigma|$  scales quadratically with  $\mathcal{L}$ , whereas base-pair degeneracy leads the replication space to display an exponential growth. Since each  $H_i$  is a binary entropy, the total entropy  $H$  satisfies  $0 \leq H \leq d$ , yielding minimum navigability of the sequence space in the absence of degeneracy (A4), and maximum navigability when all degenerated base pairs are equally probable (A4\* in our simulations).

Solid lines in Fig. S4 correspond to the analytical computation of  $|\sigma|$  (Eq. 5 and 7) for different  $H$  values and lines with data points show exhaustive numeric computations of  $|\sigma|$  for A4 and A4\*, excluding repeated sequences. It is evident that  $|\sigma|$  increases substantially when degeneracy is incorporated into the alphabet, while remaining constrained by the entropy associated  $H$ . It is important to note, however, that the analytical curve of  $|\sigma|$  for  $H = 2$  deviates from the exhaustive calculation. This is due to two simplifying assumptions: (i) the analytical model ignores the unavoidable repetition of complementary sequences; and (ii) it assumes uniform distribution of degenerated bases along the sequence, while our computational analyses reveal that the random emergence of centered segments with clustered degenerated nts further enhance the effective degeneracy and navigability of the sequence space.

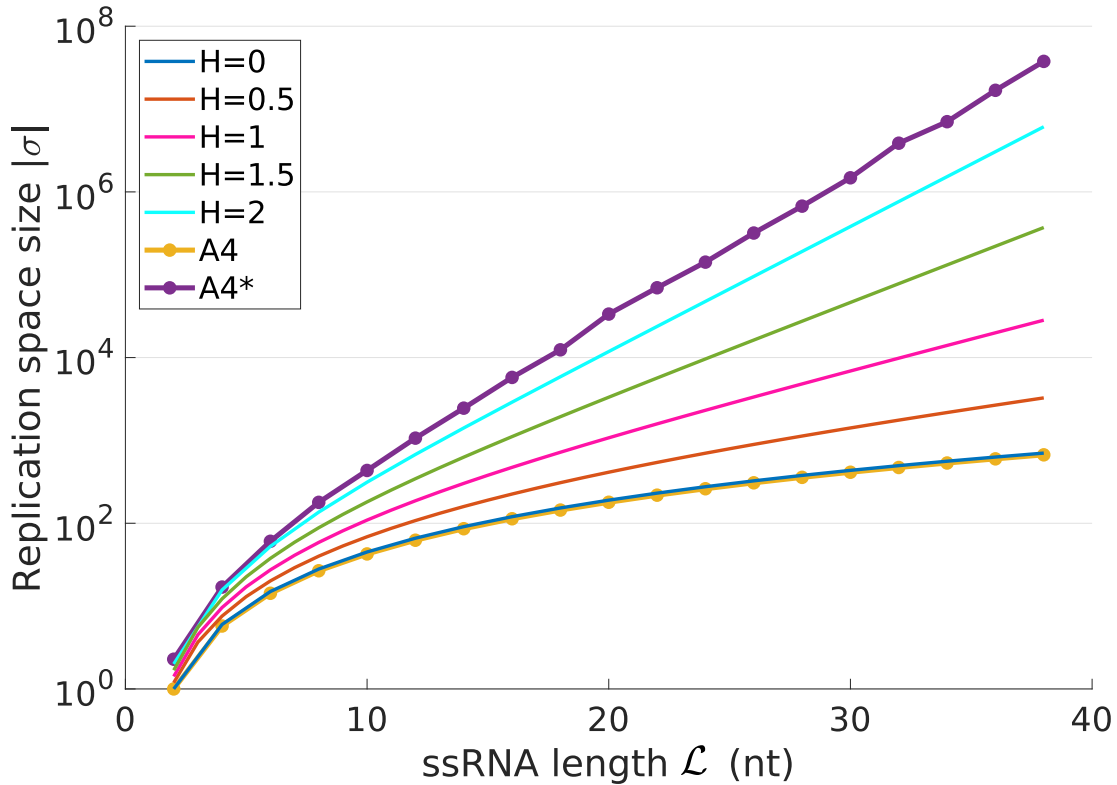

Figure S4: Dependence of the replication space size  $|\sigma|$  with the length  $\mathcal{L}$  of a ssRNA. Lines with data points show the exhaustive numeric computation of  $|\sigma|$  for A4 and A4\*, excluding repeated sequences (mean of 500 realizations, errors excluded for clarity); solid lines correspond to the analytical computation of  $|\sigma|$  for different  $H$  values (Eq. 5 for  $H = 0$  and Eq. 7 for the rest).

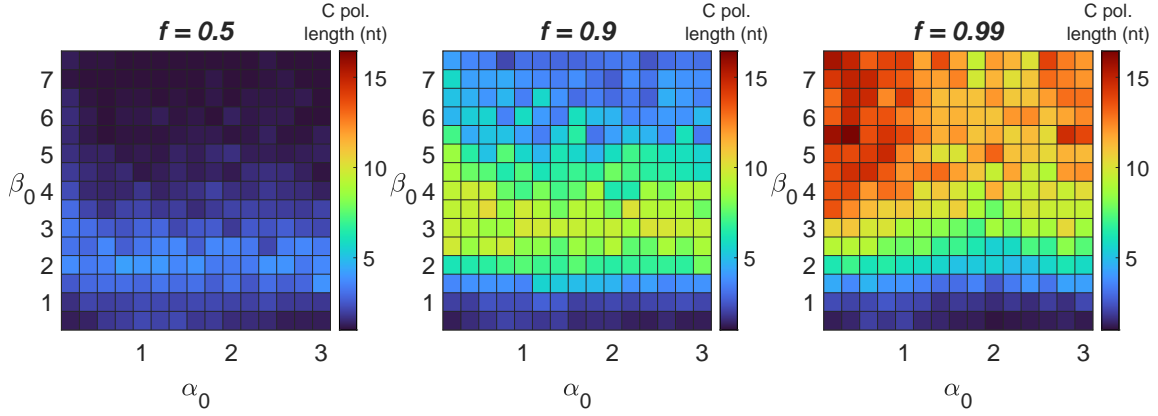

Figure S5: Dependence of the mean of maximum C polymer lengths with average interaction parameters  $\alpha_0$  and  $\beta_0$  at three different amplitude fractions  $f$  (being  $A_\alpha = f\alpha_0$  and  $A_\beta = f\beta_0$ ).  $T_\alpha = T_\beta = 2500$ . Every simulation started with a different 20 nt-long ssRNA molecule of random position and sequence, and means were calculated over 20 independent realizations for each parameter set.

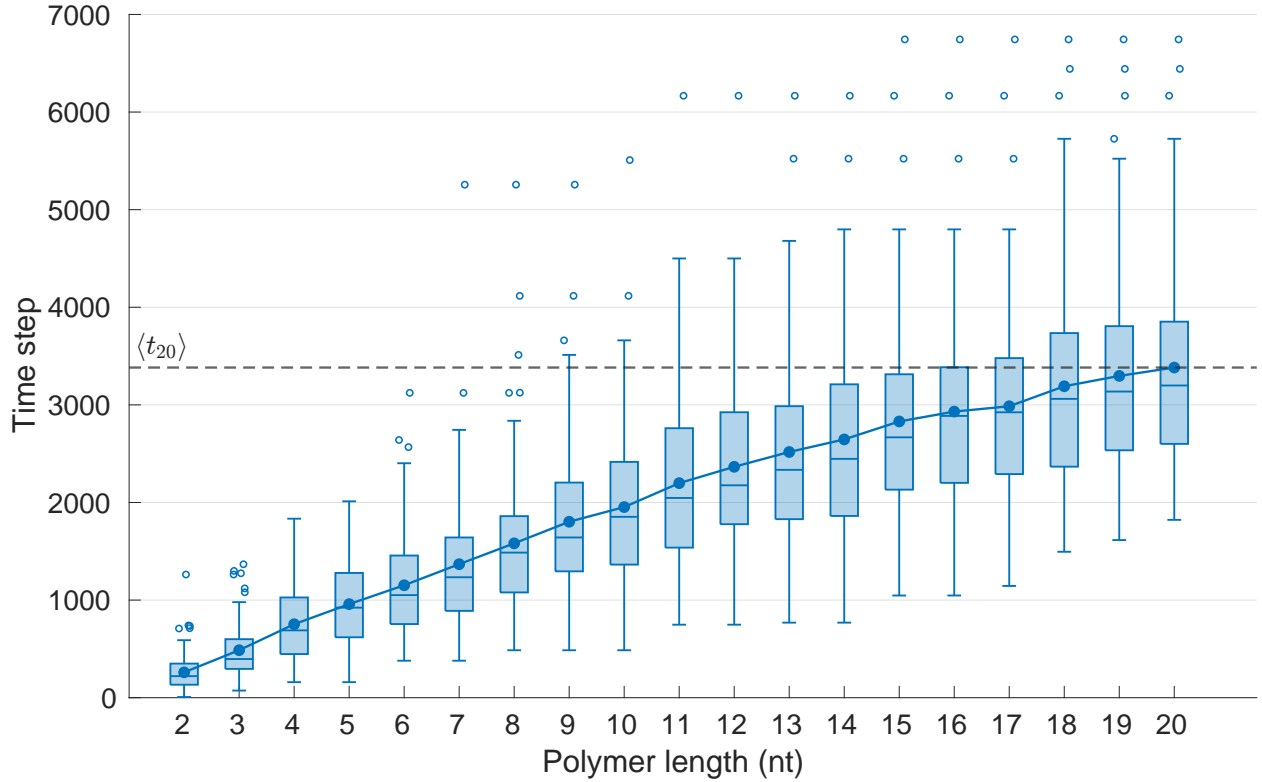

Figure S6: Number of time steps required by EarlyWorld to produce a ssRNA polymer C complementary to the original one (O), by template-dependent polymerization, as a function of its length. In particular, we measure the time step in which a polymer C of a given length appears for the first time hybridized to O in the simulation (i.e., it does not need to be released to the pool). The dashed line shows the mean time  $\langle t_{20} \rangle = 3294$  time steps to form a 20-nt long polymer C. Each box plot and mean (colored circles) were calculated using 100 independent realizations. Parameters: constant environment with  $\alpha_0 = 0.8$  and  $\beta = 6$ .

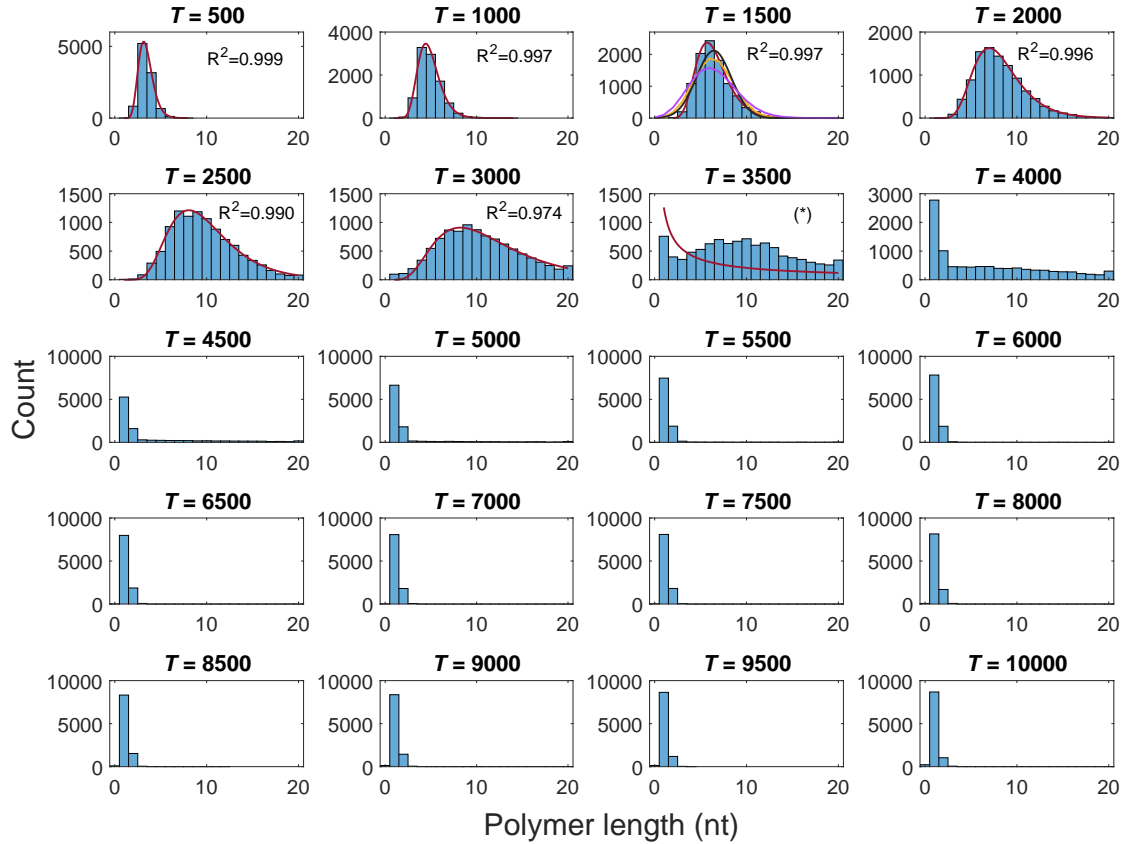

Figure S7: Distribution of maximum R polymer lengths for twenty different oscillation periods  $T = T_\alpha = T_\beta$ . Approximations to log-normal distributions are displayed in red with their corresponding  $R^2$  coefficient. In  $T = 1500$  data were also approximated to a normal distribution (black line,  $R^2 = 0.941$ ), a binomial distribution (yellow line,  $R^2 = 0.933$ ) and a Poisson distribution (pink line,  $R^2 = 0.859$ ). The log-normal distribution approximates accurately the data until a transition occurs at  $T \approx 3500$ , beyond which the distributions show first a peak in 1 nt and a long tail, and for larger values of  $T$  they finally collapse to the absence of any relevant replication. Data include  $10^4$  independent realizations for each parameter set with parameters  $\alpha_0 = 0.8$ ,  $A_\alpha = 0.5$ ,  $\beta_0 = 6$ , and  $A_\beta = 5.9$  (coinciding with those of Fig. 4B). (\*) The log-normal approximation of these data is worse than if they were approximated to a horizontal line.

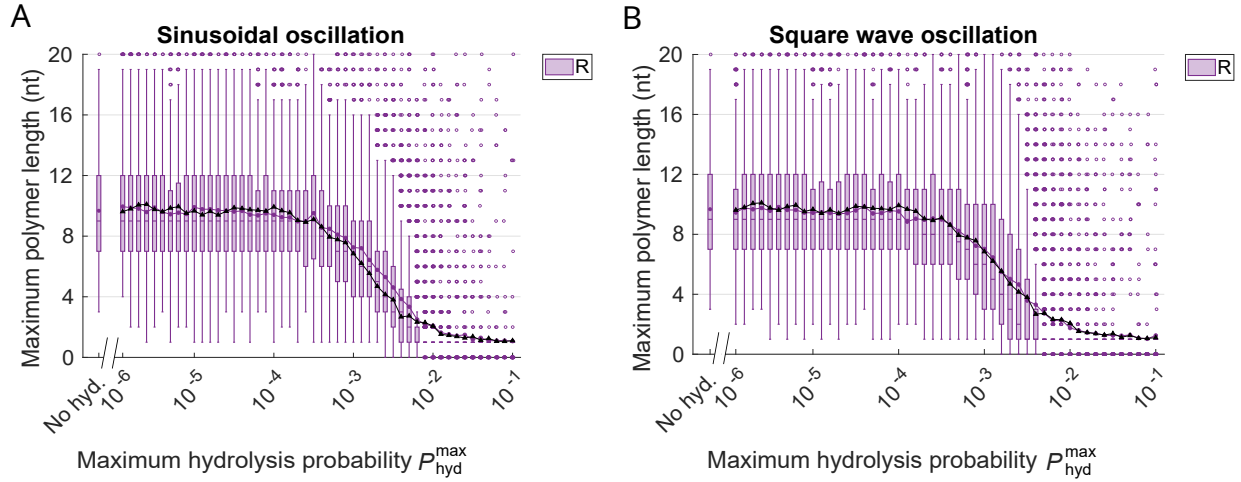

Figure S8: Distributions of maximum replicate polymer lengths for different hydrolysis probabilities in fluctuating environments. We consider oscillations of maximum hydrolysis probabilities  $P_{\text{hyd}}^{\text{max}}$  and a fixed minimum hydrolysis probability  $P_{\text{hyd}}^{\text{min}}$ . (A) The oscillation is sinusoidal (in a logarithmic scale), and follows  $\log P_{\text{hyd}} = \frac{1}{2} \log(P_{\text{hyd}}^{\text{min}} \cdot P_{\text{hyd}}^{\text{max}}) + \frac{1}{2} \log(P_{\text{hyd}}^{\text{min}}/P_{\text{hyd}}^{\text{max}}) \sin(2\pi t/T)$ . (B) The oscillation is a square wave and follows  $\log P_{\text{hyd}} = \frac{1}{2} \log(P_{\text{hyd}}^{\text{min}} \cdot P_{\text{hyd}}^{\text{max}}) + \frac{1}{2} \log(P_{\text{hyd}}^{\text{min}}/P_{\text{hyd}}^{\text{max}}) \text{sgn}(\sin(2\pi t/T))$ . Each box plot and mean (colored circles connected by lines) were calculated using 500 realizations. For comparison, the mean values of maximum replicate polymer lengths for a constant  $P_{\text{hyd}}$  are included as a black line (obtained from Fig. 4C in the main text), and the case without hydrolysis is included as the leftmost box plot. Parameters:  $\alpha_0 = 0.8$ ,  $A_\alpha = 0.5$ ,  $\beta_0 = 6$ ,  $A_\beta = 5.9$ ,  $T = T_\alpha = T_\beta = 2500$ ,  $P_{\text{hyd}}^{\text{min}} = 10^{-7}$ . Hydrolysis was introduced in the model by evaluating the probability of covalent bond breakage  $P_{\text{hyd}}$  (hydrolysis probability) of all susceptible phosphodiester bonds in each time step. Assuming that hydrolysis affects more strongly nt-nt bonds fully exposed to water (rather than those stabilized by dsRNA formation or interactions with clay), we restrict phosphodiester bond breakage to ssRNA molecules (or ssRNA fragments inside a mixed ssRNA/dsRNA molecule) freely floating in the pool. More specifically, we do not consider susceptible to hydrolysis those phosphodiester bonds joining two nts that are base-paired with their complementary ones.

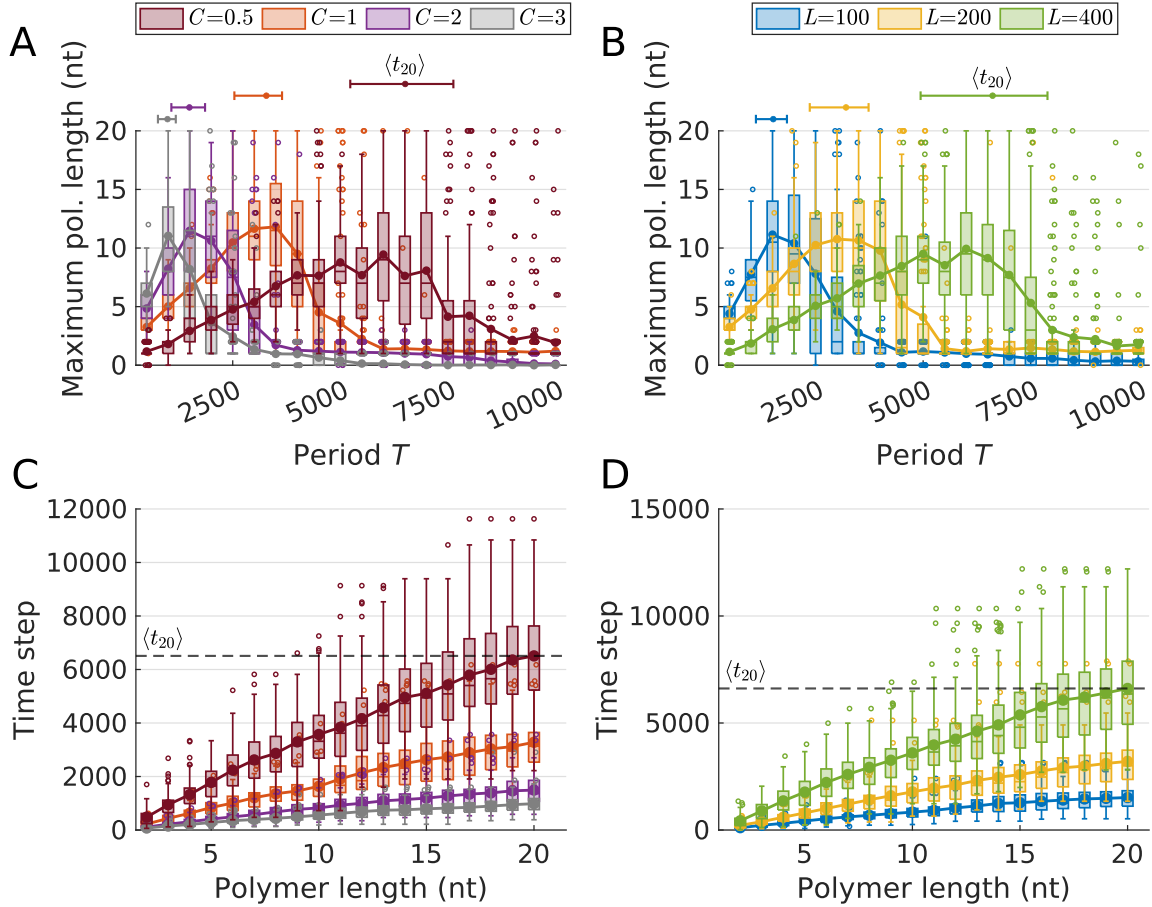

Figure S9: Effect of nucleotide concentration  $C$ —simulated by changing the number of molecules that fall into the clay per time step—and clay length  $L$  on the template-dependent replication of a ssRNA molecule adsorbed to a clay surface (comp.II). (A) Dependence of the maximum length distribution of R polymers on the oscillation period  $T = T_\alpha = T_\beta$  for different nucleotide concentrations and (B) for different clay lengths. Parameters of panels A and B:  $\alpha_0 = 0.6$ ,  $\beta_0 = 7$  and  $f = 0.99$  (coinciding with the most favorable result in Fig. 4A). The mean time to polymerize a 20-nt long ssRNA by template-dependent polymerization (obtained from panels C and D, and marked only for  $C = 0.5$  and  $L = 400$  for clarity) is displayed above the figures with 25th-75th percentiles for each concentration and clay length. Notice that the value of the oscillation period that optimizes the replication dynamics in all cases coincides with the number of simulation time steps that in average is required to form a complete 20-nt long complementary copy attached to the original O sequence. C) Number of time steps required by EarlyWorld to produce a ssRNA polymer C complementary to the original by template-dependent polymerization, as a function of its length, as in Fig. S6, for different concentrations and (D) clay lengths. Parameters of panels C and D: constant environment with  $\alpha = 0.6$  and  $\beta = 7$ . Each box plot and mean (colored circles) were calculated using 100 independent realizations.

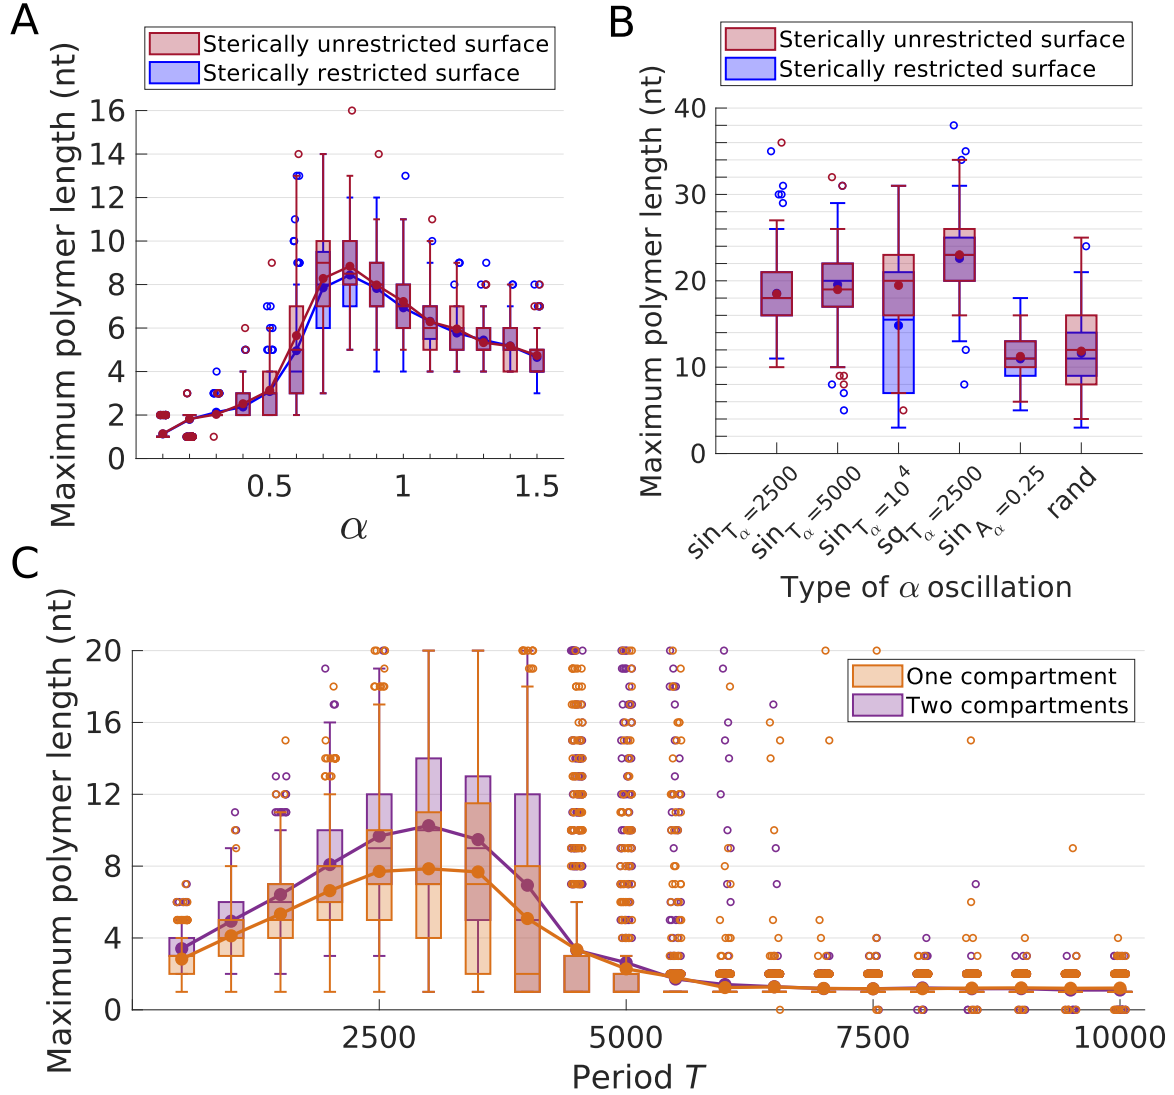

Figure S10: Efficiency of RNA polymerization and replication in different clay scenarios. (A) Maximum polymer length distributions over  $\alpha$ -constant environments when the polymerization takes place in (i) a sterically unrestricted surface (e.g., a wide internal channel, inter-particle site or external clay surface), with oscillating  $\beta$  (red), and (ii) a sterically restricted environment (e.g., an internal channel or interlayer) that is wide enough to allow ssRNA, but not dsRNA oligomers, to pass through (i.e., the standard comp.I of EarlyWorld) with  $\beta = 0$ , data taken from Fig. 2B (blue). (B) Maximum polymer length distributions for the two scenarios described in (A) over six  $\alpha$ -fluctuating environments: “sin” stands for sinusoidal oscillation, “sq” for square wave oscillation and “rand” for random fluctuation. (C) Dependence of the maximum replicate (R) polymer length distribution on the oscillation period  $T = T_\alpha = T_\beta$  when (i) both RNA polymerization and replication take place subsequently in a single, sterically unrestricted surface (one-compartment scenario as described in (i) of panel A, orange), and (ii) in the standard two-compartment model of EarlyWorld (purple, data taken from Fig. 4B). In the one-compartment simulations, the initial situation is a fully empty clay surface—instead of the initially preformed 20-nt long polymer attached to the clay in the two-compartment case—, polymerization and replication occur subsequently, the original polymer to be replicated is the first to reach a length of 20 nts, and the simulation time  $t_{\max} = 2 \times 10^4$ , starting when the original polymer is created. If not said otherwise in the axes of the different panels,  $\alpha_0 = 0.8$ ,  $A_\alpha = 0.5$ ,  $T_\alpha = 2500$ ,  $\beta_0 = 6$ ,  $A_\beta = 5.9$ ,  $T_\beta = 2500$ . Every simulation was repeated 100 times in (A) and (B), and 500 times in (C).

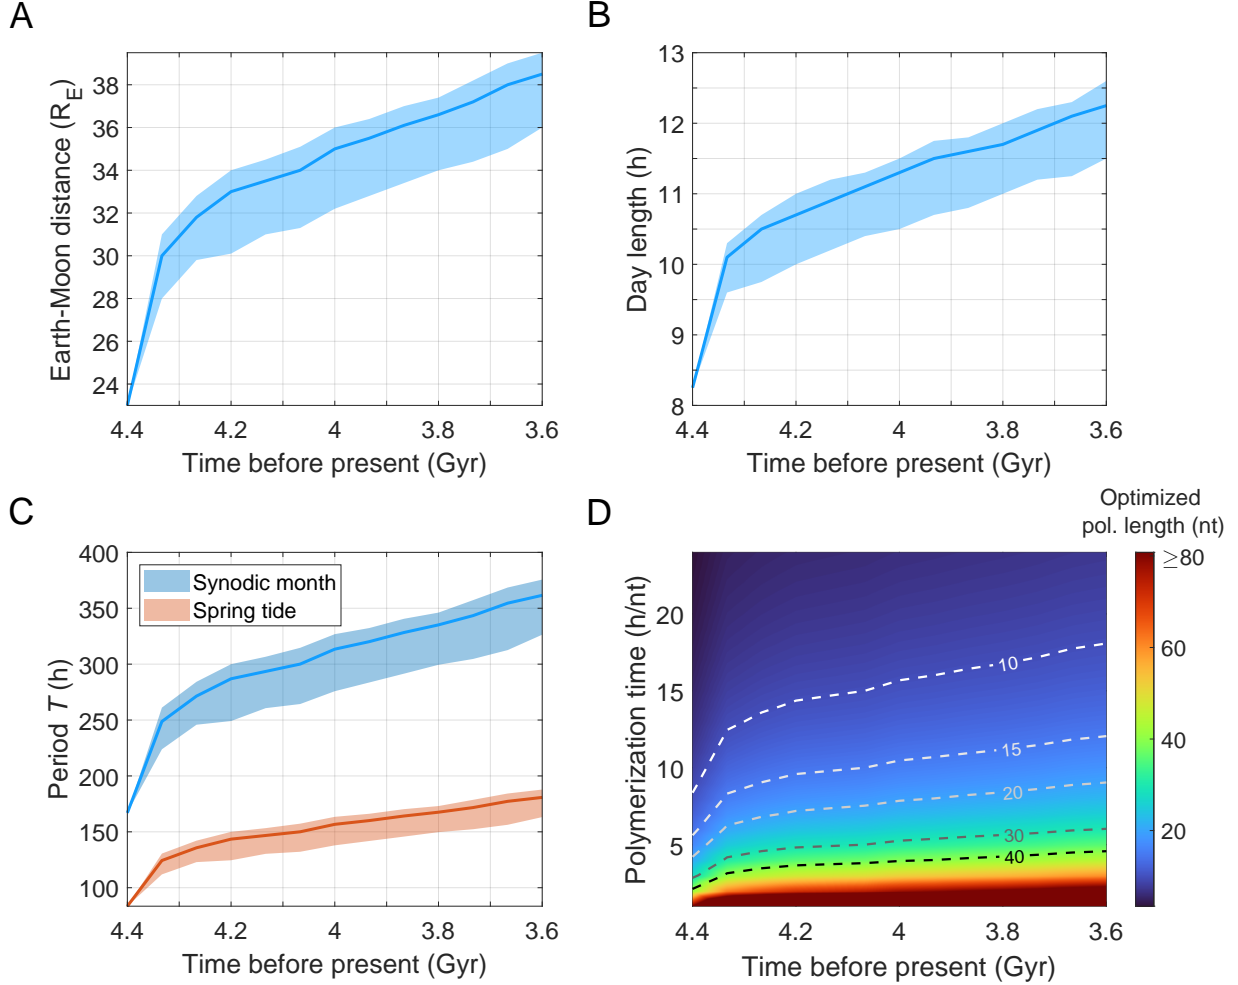

Figure S11: Evolution with time of the main astronomical data related to the Earth-Moon system, and evolution with time of the dependence of the optimized polymer length on the template-dependent polymerization time in the clay-water scenario considered in early Earth. (A) Lunar semi-major axis (measured in Earth radii  $R_E$ ). For comparison, current lunar semi-major axis is  $\sim 60R_E$ . Data in (A, B) were obtained from Fig. 3 and Fig. 5 in [12]. Bold lines in (A,B,C) represent data means, and shaded envelopes correspond to  $2\sigma$ -uncertainties. (B) Earth's length of the day. (C) Synodic month period (or lunation, or Moon phase cycle, i.e., the time between two Sun-Earth-Moon alignments, calculated applying Kepler's third law to data in panel (A) and current data, blue), and spring tide period  $T_{st}$  (i.e., the time between a Sun-Earth-Moon and a Sun-Moon-Earth alignment, orange). Current synodic month period is 29.53 days (708.72 h) and current spring tide period is 14.76 days (354.36 h, half a synodic month). (D) Dependence of the optimized polymer length  $l_{opt}$  on the template-dependent polymerization time per nt in a clay-water environment,  $t_{pol}$ , and on the time before present. The optimized polymer length is calculated as  $l_{opt} = T_{st}/t_{pol}$ . White and black dashed lines indicate  $l_{opt}$  of 10, 15, 20, 30 and 40 nts.

## References

- [1] Wei Hua Yu, Na Li, Dong Shen Tong, Chun Hui Zhou, Chun Xiang Cynthia Lin, and Chuan Yun Xu. Adsorption of proteins and nucleic acids on clay minerals and their interactions: A review. *Applied Clay Science*, 80:443–452, 2013.
- [2] Ulysse Pedreira-Segade, Jihua Hao, Angelina Razafitianamaharavo, Manuel Pelletier, Virginie Marry, Sébastien Le Crom, Laurent J Michot, and Isabelle Daniel. How do nucleotides adsorb onto clays? *Life*, 8(4):59, 2018.
- [3] Luís H de Oliveira, Pollyana Trigueiro, Baptiste Rigaud, Edson C da Silva-Filho, Josy A Osajima, Maria G Fonseca, Jean-François Lambert, Thomas Georgelin, and Maguy Jaber. When RNA meets montmorillonite: Influence of the pH and divalent cations. *Applied Clay Science*, 214:106234, 2021.
- [4] Shu Qing Zhou, Yu Qin Niu, Jia Hui Liu, Xi Xi Chen, Chun Sheng Li, Will P Gates, and Chun Hui Zhou. Functional montmorillonite/polymer coatings. *Clays and Clay Minerals*, 70(2):209–232, 2022.
- [5] Marco Franchi, James P Ferris, and Enzo Gallori. Cations as mediators of the adsorption of nucleic acids on clay surfaces in prebiotic environments. *Origins of Life and Evolution of the Biosphere*, 33:1–16, 2003.
- [6] James P Ferris. Montmorillonite-catalysed formation of RNA oligomers: the possible role of catalysis in the origins of life. *Philosophical Transactions of the Royal Society B: Biological Sciences*, 361(1474):1777–1786, 2006.
- [7] Joachim H Rosenberger, Tobias Göppel, Patrick W Kudella, Dieter Braun, Ulrich Gerland, and Bernhard Altaner. Self-assembly of informational polymers by templated ligation. *Physical Review X*, 11(3):031055, 2021.
- [8] Chrisantha Fernando, Günter Von Kiedrowski, and Eörs Szathmáry. A stochastic model of nonenzymatic nucleic acid replication: “Elongators” sequester replicators. *Journal of Molecular Evolution*, 64:572–585, 2007.
- [9] Gerard 't Hooft, William D Phillips, Anton Zeilinger, Roland Allen, Jim Baggott, François R Bouchet, Solange M G Cantanhede, Lázaro A M Castanedo, Ana María Cetto, Alan A Coley, Bryan J Dalton, Peyman Fahimi, Sharon Franks, Alex Frano, Edward S Fry, Steven Goldfarb, Karlheinz Langanke, Chérif F Matta, Dimitri Nanopoulos, Chad Orzel, Sam Patrick, Viraj A A Sanghai, Ivan K Schuller, Oleg Shpyrko, and Suzy Lidström. The sounds of science—a symphony for many instruments and voices: part ii. *Physica Scripta*, 99(5):052501, apr 2024.
- [10] L Gatlin. *Information Theory and the Living System*. Columbia University Press, 1972.
- [11] Thomas M Cover. *Elements of information theory*. John Wiley & Sons, 1999.
- [12] Mohammad Farhat, Pierre Auclair-Desrotour, Gwenaél Boué, and Jacques Laskar. The resonant tidal evolution of the Earth-Moon distance. *Astronomy & Astrophysics*, 665:L1, 2022.
